# Supplementary material for: Laser Writing of Parabolic Micromirrors with a High Numerical Aperture for Optical Trapping and Rotation
Source: arXiv:2308.06345 source file (2023-08-11)
Supplement: Supplementary file 1 [file Micromirrors_SI.pdf]

**Supplementary Material for:**

# Laser Writing of Parabolic Micromirrors with a High Numerical Aperture for Optical Trapping and Rotation

T. Plaskocinski,[1] Y. Arita,[1] G. D. Bruce,[1] S. Persheyev,[1] K. Dholakia,[1,2,3] A. Di Falco,[1,a)] and H. Ohadi[1,b)]

(Authors to whom correspondence should be addressed: adf10@st-andrews.ac.uk, ho35@st-andrews.ac.uk)

[1)] *SUPA, School of Physics and Astronomy, University of St Andrews, North Haugh, St. Andrews, Fife, KY16 9SS, United Kingdom*

[2)] *School of Biological Sciences, University of Adelaide, Adelaide, South Australia, Australia*

[3)] *Centre of Light for Life, University of Adelaide, Australia*

(Dated: 10 August 2023)

[a)] Electronic mail: adf10@st-andrews.ac.uk

[b)] Electronic mail: ho35@st-andrews.ac.uk

## I. SUPPLEMENTARY VIDEOS

SV1 – Trapping handover from microscope objective to micromirror trap.

SV2 – Rotation of vaterite with the objective.

SV3 – Counter-rotation of vaterite with mirror.

SV4 – Movement of the stage while trapping a particle, showing it is trapped only using the micromirror trap.

## II. SUPPLEMENTARY FIGURES

S1 – Micromirror array, and the typical parameters used in fabrication.

S2 – Gold channel fabricated by direct laser writing.

S3 – Scanning scheme used to measure the micromirror profile and profile of micromirror with x and z axes equal .

S4 – Relationship between exposure time, laser power, and the depth and diameter of micromirrors.

S5 – Relationship between laser position, power, and the depth and diameter of micromirrors, along with geometry used.

S6 – Relationship between exposure time, laser power, pulse repetition rate, and the depth and diameter of micromirrors.

S7 – Micromirror ellipticity.

S8 - Microfluidic chamber scheme.

S9 - Estimation of the size of the beam incident on the micromirrors.

S10 - Image and diagram of beam reflected by micromirror.

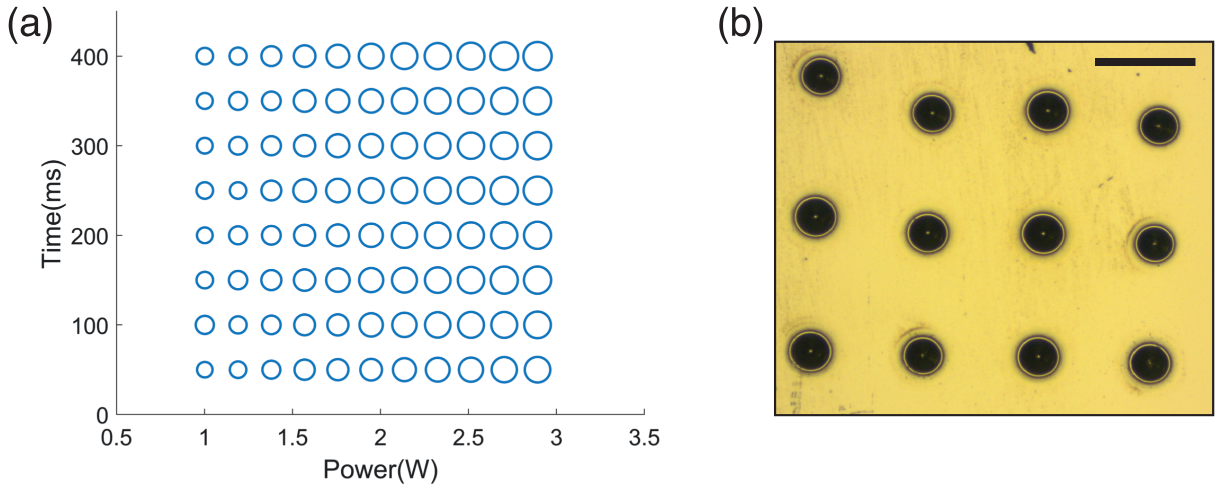


S 1. (a) Fabrication parameters of a typical array of mirrors and b) microscope image of a gold-coated array. The scale bar is 200 μm.

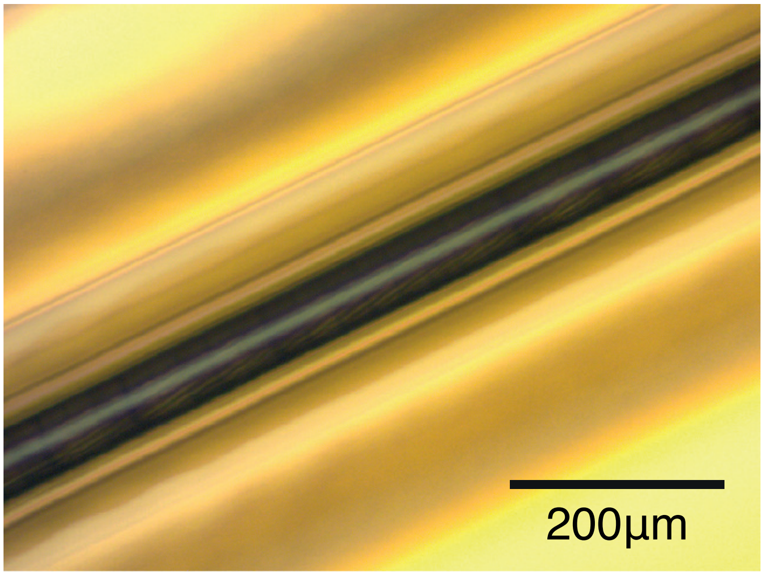


S 2. Gold channel fabricated by direct laser writing.

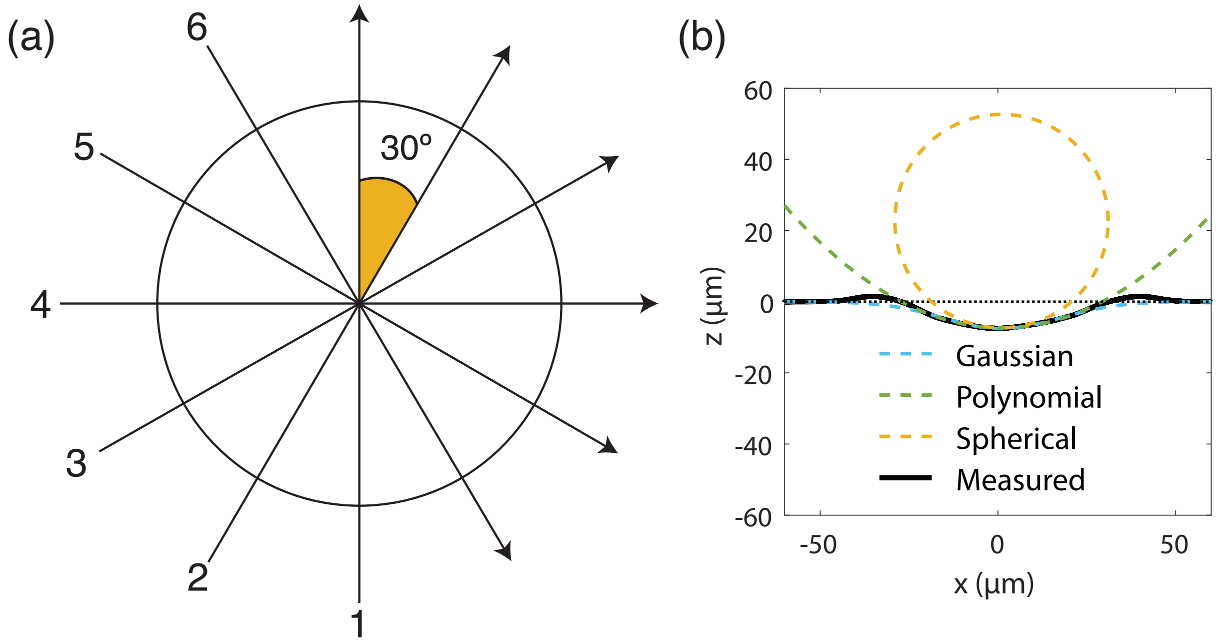


S 3. (a) Geometry of the scans across the mirror used for trapping, which were then averaged out to give the profile shown in (b) the profile of the micromirror with x and z axes equal. The circle used for the spherical fit has a 30 μm diameter.

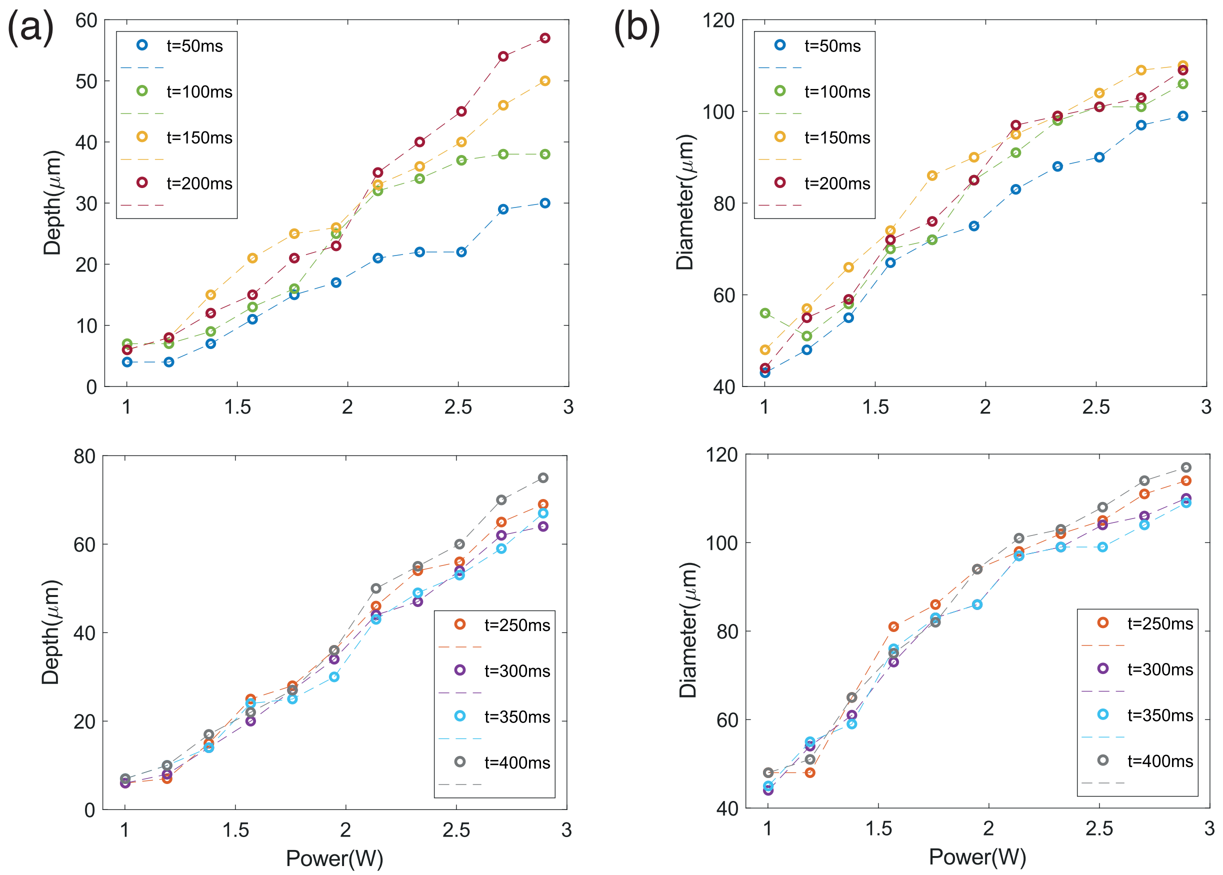


S 4. Relationship between the time of exposure, power of the laser, and the resulting (a) diameter and (b) depth of the micromirrors.

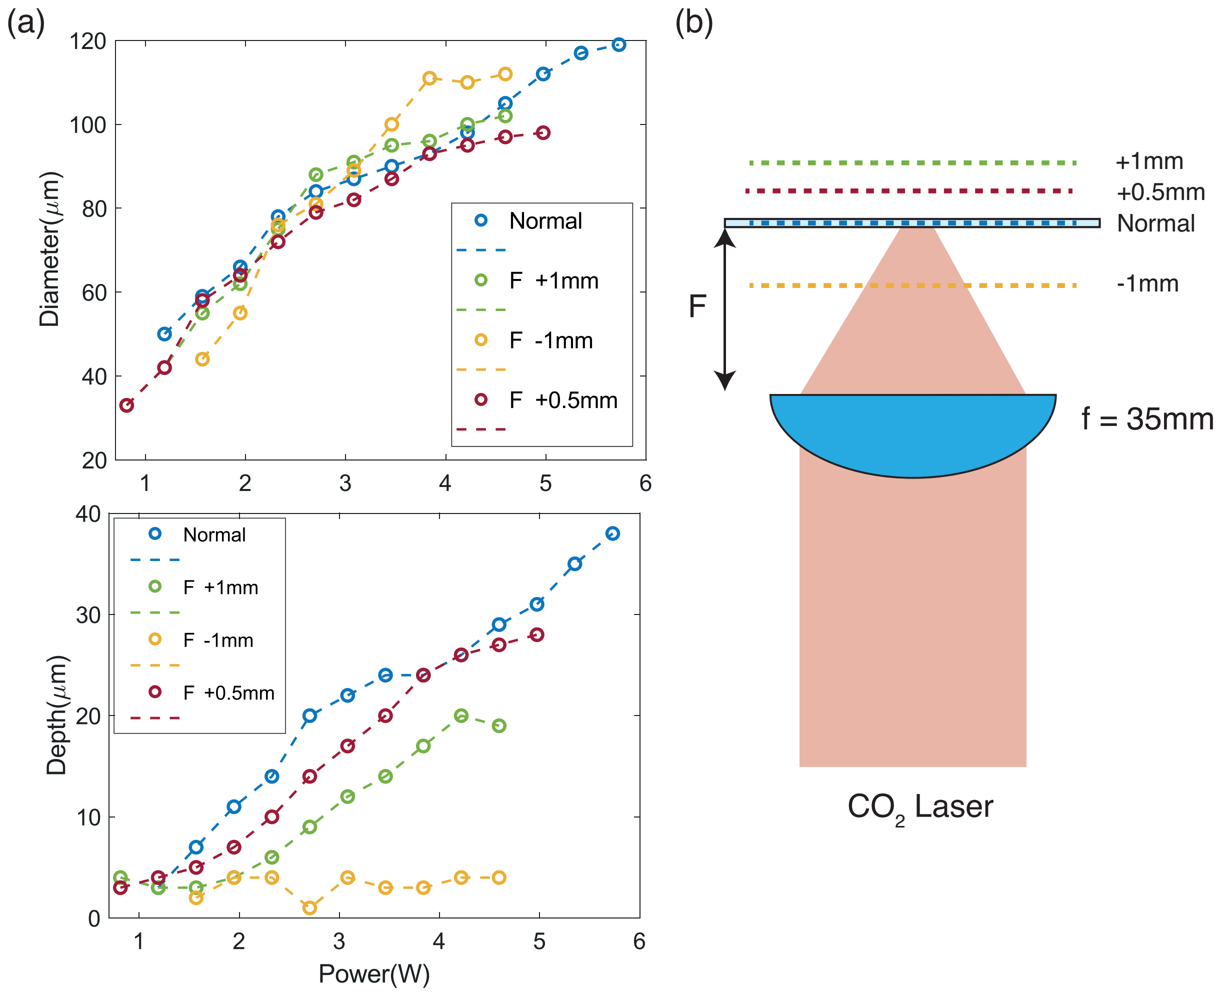


S 5. (a) Relationship between the location of the focal point of the laser relative to ntethe plane of the glass slide, power of the laser, and the resulting diameter and depth of the micromirror for a 20 ms pulse length. (b) Sketch of the geometry, the glass slide would be displaced to achieve different focusing planes.

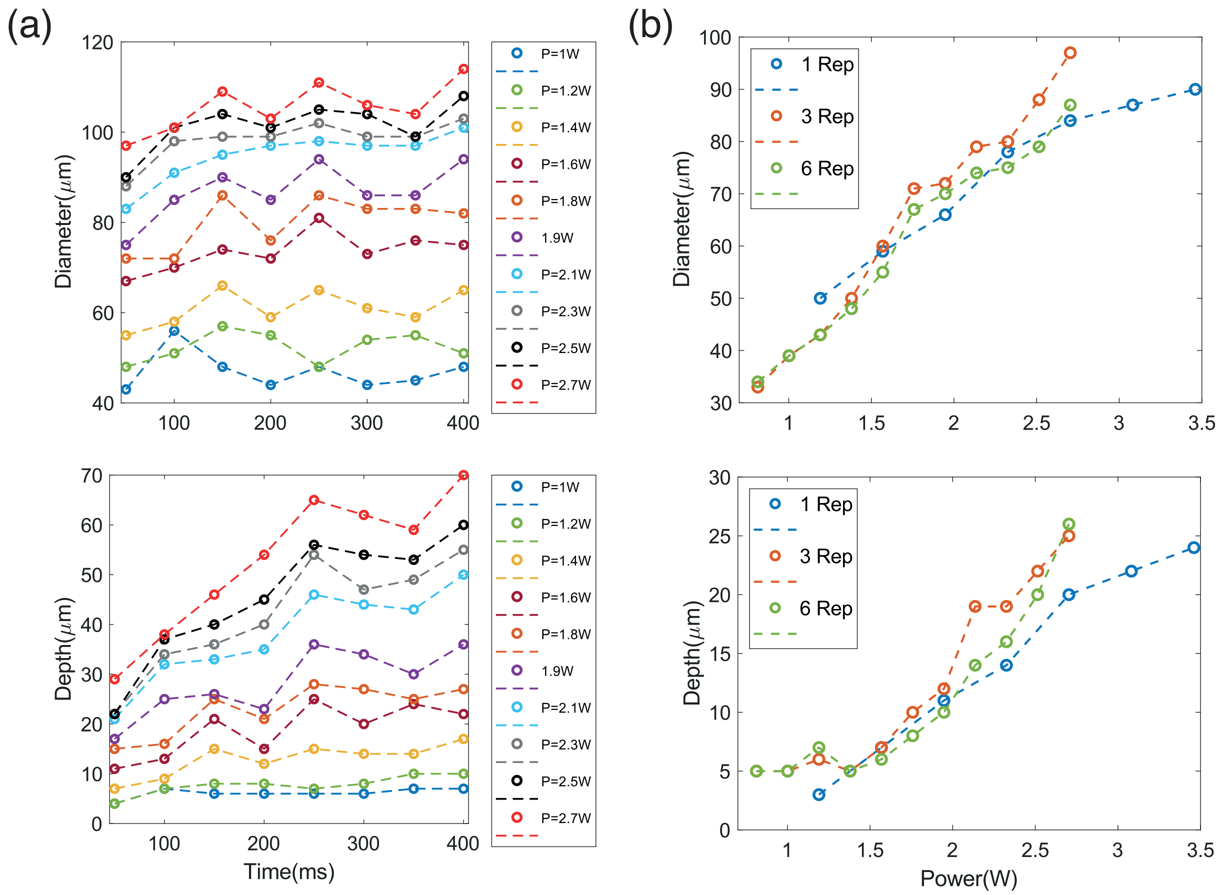


S 6. (a) Relationship between time and diameter, depth at different powers. (b) Relationship between repetition rate and diameter, depth at different powers.

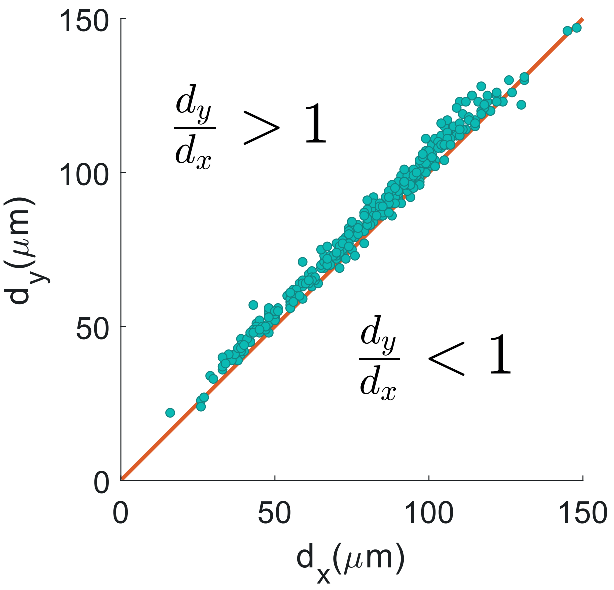


S 7. Ellipticity of the micromirrors, explaining discrepancies between trapping stiffness in x and y directions.

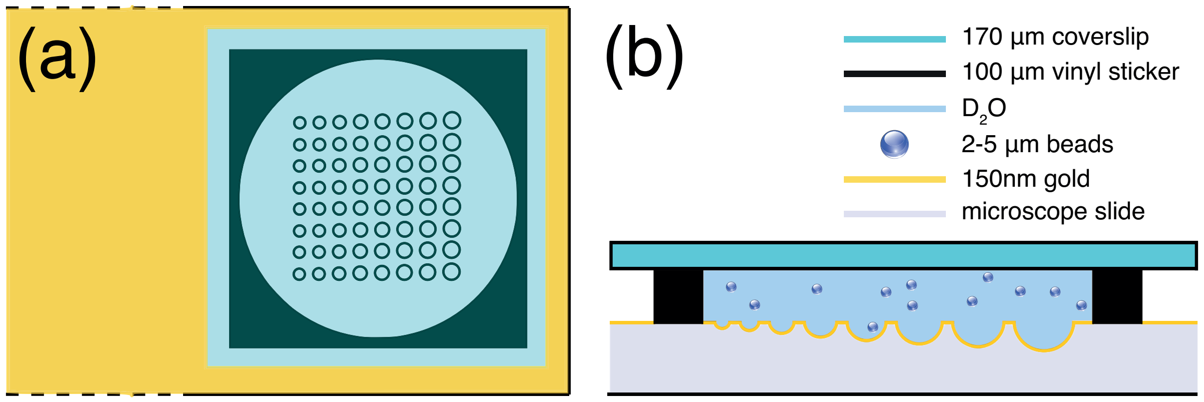


S 8. Microfluidic chamber on top of the gold-coated slide, consisting of a black vinyl spacer and a glass coverslip adhered using nail varnish from (a) above and (b) side.

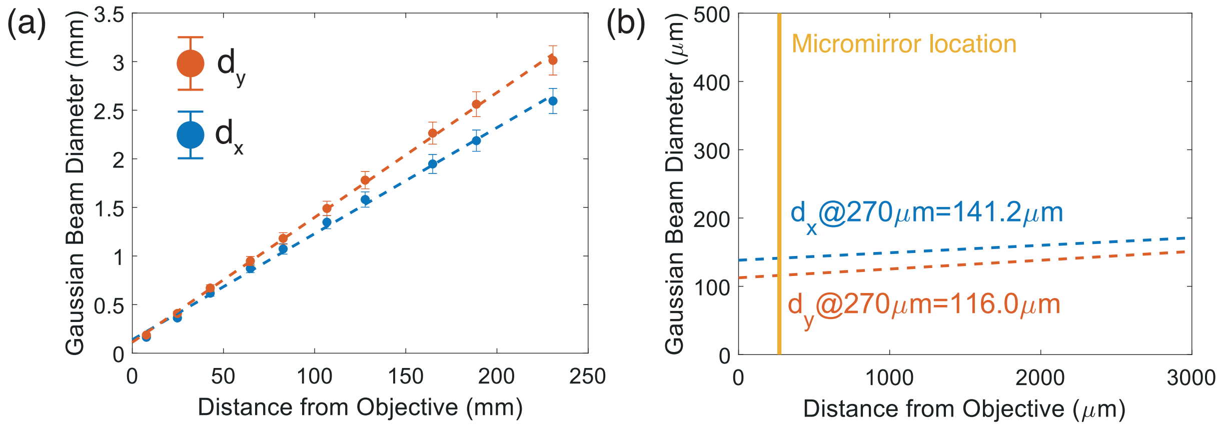


S 9. (a) Beam size estimation, with (b) zooming in on the section where the micromirror traps would have been illuminated by the beam.

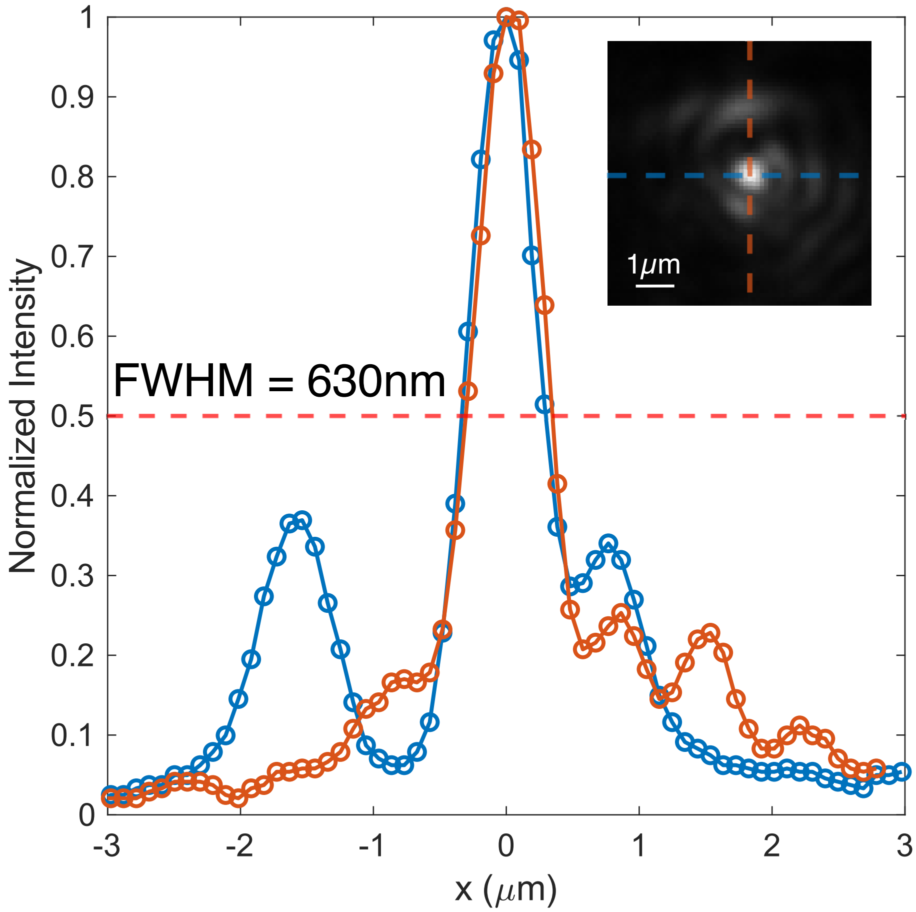


S 10. Horizontal and vertical profile of the spot formed by the micromirror. Inset shows image used.
